# Supplementary material for: Learning Task Priorities from Demonstrations
Source: arXiv:1707.06791 source file (2018-11-20)
Supplement: Supplementary file 1 [file appendixCandidateProj.tex]

%\section{Obtaining angular velocity using linear operators}
\section*{Appendix B: Obtaining angular velocity using linear operators}
\label{app:TPorientation}

From Equation (9), angular velocity is obtained using the operator ${\mathrm{vec}(\mb{\epsilon}_{t}*\mb{\bar{\epsilon}}_{t-1})}$, whose non-linearity is incompatible with the structure of TP-GMM parameterization. We can however employ unit quaternion properties (Appendix \iffalse \ref{app:Quat}\fi A) to simplify this operator. For any unit quaternion, $\mathrm{vec}(\mb{\epsilon})$ can be replaced by the matrix operation $\mathrm{vec}(\mb{\epsilon}) = \left[ \begin{matrix} \mb{0}^{3\times1} & \mb{I}^{3\times3} \end{matrix} \right] \mb{\epsilon}$, allowing us to rewrite (9) as
\begin{equation}
\mb{\omega}_t = \left[ \begin{matrix} \mb{0}^{3\times1} & \mb{I}^{3\times3} \end{matrix} \right] (\mb{\epsilon}_{t}*\mb{\bar{\epsilon}}_{t-1})\frac{1}{\Delta t}.
\end{equation}

The quaternion product $ \mb{\epsilon}_{t}*\mb{\bar{\epsilon}}_{t-1} $ can also be replaced by a matrix product using the quaternion matrices. We take advantage of matrix $\HRight$ from \eqref{eq:Hamiltons} that allows for changing the order in which two quaternions are multiplied without changing the resulting orientation. We can thus write
\begin{align}
&\mb{\epsilon}_t*\mb{\bar{\epsilon}}_{t-1} = \HRight(\mb{\bar{\epsilon}}_{t-1})\>\mb{\epsilon}_t \\
\Rightarrow & \>\> \mb{\omega}_t = \left[ \begin{matrix} \mb{0}^{3\times1} & \mb{I}^{3\times3} \end{matrix} \right] \HRight(\mb{\bar{\epsilon}}_{t-1})\>\mb{\epsilon}_t\frac{1}{\Delta t}.
\label{eq:quatProdHRight}
\end{align}
Defining, for any matrix $\mb{M}\!\in\!\mathbb{R}^{4\times4}$, ${ \mb{M^*} = \left[ \begin{matrix} \mb{0}^{3\times1} &  \mb{I}^{3\times3} \end{matrix} \right] \mb{M}}$, Eq.  \eqref{eq:quatProdHRight} yields
\begin{align}
\mb{\omega}_t & = \HRightVec\!(\mb{\bar{\epsilon}}_{t-1})\>\mb{\epsilon}_t \frac{1}{\Delta t}\>.
\label{eq:linearW}
\end{align}
Note that other operations can be used in place of Eq. (9) to obtain an angular velocity, namely the logarithmic map of the unit quaternion (see \cite{Ude14ICRA} for a comparison with (9)). However, the linear structure of Eq. \eqref{eq:linearW} makes (9) a convenient form for the TP-GMM parameterization.
