# Supplementary material for: Learning Task Priorities from Demonstrations
Source: arXiv:1707.06791 source file (2018-11-20)
Supplement: Supplementary file 2 [file appendixDSGMR.tex]

\section{Statistical Dynamical Systems}
\label{app:DynamicalSytems}
In \cite{Silverio15}, we introduced a statistical dynamical system approach for learning end-effector poses. The end-effector is modeled as a unit mass spring-and-damper system, whose pose is governed by a set of second order linear differential equations
\begin{equation}
\label{eq:positionMSD}
\mb{\ddot{x}} = \mb{K}_p(\mb{\hat{x}}-\mb{x}) - \mb{K}_v \mb{\dot{x}},
\end{equation}
\begin{equation}
\label{eq:orientationMSD}
\dot{\mb{\omega}} = \mb{K}_o \;2\> \mathrm{log}(\mb{\hat{\epsilon}}*\mb{\bar{\epsilon}}) - \mb{K}_\omega \mb{\omega} ,
\end{equation}
where $\mb{K}_p$, $\mb{K}_o$ are stiffness matrices and $\mb{K}_v$, $\mb{K}_\omega$ are damping matrices. The matrices are selected manually according to the desired compliance of the movement and poses are learned as attractors which are computed with
\begin{equation}
\mb{\hat{x}} = \mb{K}^{-1}_p\mb{\ddot{x}}+ \mb{K}^{-1}_p \mb{K}_v \mb{\dot{x}} + \mb{x}.
\label{eq:positionAttractor}
\end{equation}
\begin{equation}
\label{eq:orientationAttractor}
\mb{\hat{\epsilon}} = \mathrm{exp}\left(\frac{1}{2}\mb{K}_o^{-1}\dot{\mb\omega} + \frac{1}{2}\mb{K}_o^{-1}\mb{K}_\omega \mb\omega\right) * \mb{\epsilon} \>.
\end{equation}
Alternatively the gain matrices can be estimated from the allowed variability of the movement encoded in the probabilistic model, see \cite{Calinon14ICRA}.

In \eqref{eq:orientationMSD} we employed the logarithm of a unit quaternion, ${\mathrm{log}\!:S^3\rightarrow\mathbb{R}^3}$, which is given by \cite{Ude14ICRA}
\begin{equation}
\label{eq:quaternionLog}
\mathrm{log}(\mb \epsilon ) = \left\{ \begin{array}{l l}
\arccos(v)\frac{\mb{u}}{||\mb{u}||}, & \mb{u}\neq 0\\
$[$0 \;\; 0 \;\; 0$]$^\trsp, & \mathrm{otherwise}.
\end{array} \right.
\end{equation}
The term $2\>\mathrm{log}(\mb{\hat{\epsilon}} * \mb{\bar{\epsilon}})$ returns the angular velocity that rotates $\mb{\epsilon}$ into $\mb{\hat{\epsilon}}$ in the unit time.
In \eqref{eq:orientationAttractor} we used the exponential of a quaternion, ${\mathrm{exp}\!:\mathbb{R}^3 \rightarrow 	S^3}$%, converts an orientation in axis-angle representation into a unit quaternion
\begin{equation*}
\mathrm{exp}(\mb r ) = \left\{ \begin{array}{l l}
\left[ \mathrm{cos}(||\mb{r}||) \hspace*{0.4cm} \mathrm{sin}(||\mb{r}||)\frac{\mb{r}^\trsp}{||\mb{r}||}\right]^\trsp, & \mb{r}\neq 0\\
\left[1 \;\; 0 \;\; 0 \;\; 0\right]^\trsp, & \mathrm{otherwise},
\end{array} \right.
\end{equation*}
where $\mb{r}\in\mathbb{R}^3$. % is a vector that represents an orientation in axis-angle notation.
For $||\mb{r}||<\pi$ the two mappings are bijective and inverse to each other.
