# Supplementary material for: Learning Task Priorities from Demonstrations
Source: arXiv:1707.06791 source file (2018-11-20)
Supplement: Supplementary file 3 [file appendixIK.tex]

\section{Inverse Kinematics Preliminaries}
\label{app:IK}

Forward kinematics maps joint values to end-effector poses with respect to a robot's base
\begin{equation}
	\mb{x}_t \!=\! f(\mb{q}_t),
	\label{eq:FK}
\end{equation}
where $ \mb{x}_t \in \mathbb{R}^6$ and $\mb{q}_t \in \mathbb{R}^{N_q}$ denote pose and joint values at $ t $,  for a robot with $N_q$ DoF. Differentiating \eqref{eq:FK} yields the differential kinematics equation
\begin{equation}
	\dot{\mb{x}}_t \!=\! \mb{J}(\mb{q}_t) \; \dot{\mb{q}}_t,
	\label{eq:FKJacobianDef}
\end{equation}
%
%where $\mb{x}_t$, $\dot{\mb{x}}_t$ represent a link pose and velocity (typically the end-effector), , $\dot{\mb{q}}_t$ are the vectors of joint positions and velocities for a robot with $N_q$ DOFs and $\mb{J}(\mb{q}_t)$ is a Jacobian matrix.
where $\mb{J}(\mb{q}_t)$ is the Jacobian matrix of the end-effector. This matrix is typically comprised of two block matrices (dropping the dependencies on $\mb{q}$ and $t$, from now on):
\begin{equation}
\dot{\mb{x}} = \mb{J} \>\dot{\mb{q}}
\iff
\left[\begin{matrix} \dot{\mb{p}} \\ \mb{\omega}	\end{matrix}\right] = \left[\begin{matrix} \mb{J}_p \\ \mb{J}_o \end{matrix} \right] \dot{\mb{q}},
\label{eq:Jacobian}
\end{equation}
where $\mb{J}\in\mathbb{R}^{6\times N_q}$ is the so-called geometric Jacobian\footnote{The geometric Jacobian maps $\dot{\mb{q}}$ to $\mb{\omega}$, while the analytical Jacobian maps $\dot{\mb{q}}$ to the rates of other - minimal - representation of orientation, such as Euler angles \cite{Siciliano09Book}.}, consisting of two sub-matrices $\mb{J}_p\in \mathbb{R}^{3\times N_q}$, $\mb{J}_o\in \mathbb{R}^{3\times N_q}$ which map joint velocities to the end-effector linear and angular velocities, $\dot{\mb{p}}\in \mathbb{R}^3$, $\mb{\omega}\in \mathbb{R}^3$.

The inverse kinematics problem consists of finding a configuration $ \mb{q} $ for the robot that leads to a desired end-effector pose $ \mb{x} $. This problem is usually solved through inverse differential kinematics: for a motion trajectory assigned to the end-effector in terms of $ \dot{\mb{x}} $, we would like to find $ \dot{\mb{q}} $ that reproduces the given trajectory. In the case of redundant manipulators ($ N_q > 6 $), as the ones we consider here, there are infinite solutions for $ \dot{\mb{q}} $ so this problem is treated from an optimization perspective as the minimization of the $L_2$-norm of the residuals:
\begin{equation}
\mb{\hat{\dot{\mb{q}}}} = \arg\underset{\dot{\mb{q}}}{\min} {\|\dot{\mb{x}}-\mb{J}\dot{\mb{q}}\|}_2 = \arg\underset{\dot{\mb{q}}}{\min} {(\dot{\mb{x}}-\mb{J}\dot{\mb{q}})}^\trsp\!(\dot{\mb{x}}-\mb{J}\dot{\mb{q}}).
\label{eq:IKoptimization}
\end{equation}
The solution to this problem corresponds to the minimum-norm joint velocities and is given by:
\begin{equation}
\mb{\hat{\dot{\mb{q}}}} = \mb{J}^\psin \dot{\mb{x}}, % + \mb{N} \dot{\mb{q}}_0,%g(\mb{q}),
\label{eq:IKsol}
\end{equation}
where
\begin{equation}
	\mb{J}^\psin=\mb{J}^\trsp {\big(\mb{J}\mb{J}^\trsp\big)}^{-1}
	\label{eq:pinvJ}
\end{equation}
is the right pseudoinverse of the Jacobian matrix. Numerical integration of \eqref{eq:IKsol} yields joint references whose tracking fulfills the task. Moreover, the redundancy of the robot allows for generating internal motions in the manipulator without changing the resulting end-effector velocity. The solution is then given by:
\begin{equation}
\mb{\hat{\dot{\mb{q}}}} = \mb{J}^\psin \dot{\mb{x}} + \mb{N} \dot{\mb{q}}_0,%g(\mb{q}),
\label{eq:generalIKsol}
\end{equation}
where
\begin{equation}
	\mb{N} = \mb{I} - \mb{J}^\psin \mb{J},
\end{equation}
is the null-space projection operator and $\dot{\mb{q}}_0$ is a secondary objective that will not affect the principal $L_2$-norm minimization objective.

Another possible solution to \eqref{eq:IKoptimization} is given by 
\begin{equation}
\mb{\hat{\dot{\mb{q}}}} = {\big(\mb{J}^\trsp\mb{J}\big)}^{-1}\mb{J}^\trsp \dot{\mb{x}}, % + \mb{N} \dot{\mb{q}}_0,%g(\mb{q}),
\label{eq:IKsolLeft}
\end{equation}
where $ {\big(\mb{J}^\trsp\mb{J}\big)}^{-1}\mb{J}^\trsp $ is the left pseudo-inverse of $ \mb{J} $. This solution, however, does not correspond to the minimum-norm joint velocities.
%\subsection{Linear Quadratic Control}
