# Supplementary material for: Learning Task Priorities from Demonstrations
Source: arXiv:1707.06791 source file (2018-11-20)
Supplement: Supplementary file 4 [file appendixQuat.tex]

\section{Unit Quaternion Preliminaries}
\label{app:Quat}

A unit quaternion $\mb{\epsilon}\in \mathcal{S}^{3}$  % (with $\mathcal{S}^{3}$ being the unit hypersphere of $\mathbb{R}^{4}$)
is defined by $\mb{\epsilon} = \left[ \epsilon_0 \>\> \epsilon_1 \>\> \epsilon_2 \>\> \epsilon_3 \right]^\trsp = \left[ v \>\> \mb{u}^\trsp \right]^\trsp$, where $v\in\mathbb{R}$ and $\mb{u}\in\mathbb{R}^{3}$, following the notation used by \cite{Ude14ICRA}, are the real and vector parts of the quaternion. The conjugate of a unit quaternion is denoted by $ \mb{\bar{\epsilon}} = \left[u \>\> -\mb{u}^\trsp \right]^\trsp $. As the name implies, unit quaternions have unitary norm, i.e., $ v^2+\mb{u}^\trsp\mb{u} = \epsilon_0^2 + \epsilon_1^2 + \epsilon_2^2 + \epsilon_3^2 =1 $. 

\subsubsection*{Composition of unit quaternions}

Similarly to the product between rotation matrices, the quaternion product is in general non-commutative. It is given by
\begin{equation}
\mb{\epsilon}_1 * \mb{\epsilon}_2 =
\begin{bmatrix}
v_1v_2 - \mb{u}^\trsp_1\mb{u}_2 \\
v_1\mb{u}_2 + v_2\mb{u}_1 + \mb{u}_1\times\mb{u}_2
\end{bmatrix}\!\!,
\label{eq:quaternionProd}
\end{equation}
and it can be interpreted as a rotation operator: it rotates the frame whose orientation is described by $\mb{\epsilon}_2$ by the rotation defined by $\mb{\epsilon}_1$. Moreover, the quaternion product $ \mb{\epsilon}_1 * \mb{\bar{\epsilon}}_2 $ yields the quaternion that rotates $ \mb{\epsilon}_2 $ into $ \mb{\epsilon}_1 $.

\subsubsection*{Quaternion matrix}

The product between two quaternions $\mb{\alpha} = \left[\alpha_0 \> \alpha_1 \> \alpha_2 \> \alpha_3 \right]^\trsp$ and $\mb{\beta} = \left[\beta_0 \> \beta_1 \> \beta_2 \> \beta_3 \right]^\trsp$ can also be written in matrix form by resorting to Hamilton operators (quaternion matrices):

\begin{equation}
\mb{\alpha}*\mb{\beta} = \HLeft(\mb{\alpha})\mb{\beta} = \HRight(\mb{\beta})\mb{\alpha},
\label{eq:quatProdComut}
\end{equation}
with Hamilton operators $\HLeft$, $\HRight$ defined by (see also \cite{AdornoThesis})
\begin{equation}
\HLeft(\mb{\alpha}) \! = \!\! \left[\begin{smallmatrix}
\alpha_0 & -\alpha_1 & -\alpha_2 & -\alpha_3 \\
\alpha_1 &  \alpha_0 & -\alpha_3 &  \alpha_2 \\
\alpha_2 &  \alpha_3 &  \alpha_0 & -\alpha_1 \\
\alpha_3 & -\alpha_2 &  \alpha_1 &  \alpha_0 \\
\end{smallmatrix} \right]\!\!,
\HRight(\mb{\beta}) \! = \!\! \left[ \begin{smallmatrix}
\beta_0 & -\beta_1 & -\beta_2 & -\beta_3 \\
\beta_1 &  \beta_0 &  \beta_3 & -\beta_2 \\
\beta_2 & -\beta_3 &  \beta_0 &  \beta_1 \\
\beta_3 &  \beta_2 & -\beta_1 &  \beta_0 \\
\end{smallmatrix} \right]\!\!.
\label{eq:Hamiltons}
\end{equation}

Notice the commutativity between $\HLeft$ and $\HRight$ in \eqref{eq:quatProdComut}. Even though the quaternion product is not commutative,  Hamilton operators commute between them. This result is useful when we want to change the order of the quaternions being multiplied %using matrix algebra
without affecting the resulting orientation.
