# Supplementary material for: Learning Task Priorities from Demonstrations
Source: arXiv:1707.06791 source file (2018-11-20)
Supplement: Supplementary file 5 [file appendixAngVel.tex]

\section{Approximations of the angular velocity}
\label{app:angVelApprox}
The angular velocity that rotates a rigid body from $\mb{\epsilon}_{t-1}$ to $\mb{\epsilon}_{t}$ in $\Delta t$ can also be computed using \eqref{eq:quaternionLog},

\begin{equation}
\mb{\omega}= \frac{2\> \mathrm{log}(\mb{\epsilon_t} * \mb{\bar{\epsilon}_{t-1}})}{\Delta t} \>,
\label{eq:wFromlogMap}
\end{equation}
Replacing \eqref{eq:wFromlogMap} in \eqref{eq:IKsolOrientation}, and making $\mb{\dot{q}}_t\approx\frac{\mb{q}_t - \mb{q}_{t-1}}{\Delta t}$, \eqref{eq:IKsolOrientation} becomes 
\begin{align}
\frac{\mb{q}_t - \mb{q}_{t-1}}{\Delta t} & = \mb{J_o}^\psin(\mb{q}_{t-1}) \>\frac{2\>\mathrm{log}(\mb{\epsilon}_t * \mb{\bar{\epsilon}}_{t-1})}{\Delta t}
\\	
\iff\quad
\mb{q}_t & =  \mb{J_o}^\psin(\mb{q}_{t-1}) \> 2\>\mathrm{log}(\mb{\epsilon}_t * \mb{\bar{\epsilon}}_{t-1}) + \mb{q}_{t-1} \>.
\end{align}
The non-linear relation between $\mb{q_t}$ and $\mb{\epsilon_t}$ (through the logarithmic map) does not comply with the affine structure of TP-GMM, therefore we did not consider this solution.
